# Supplementary material for: Monitoring the orientation of rare-earth-doped nanorods for flow shear tomography
Source: arXiv:1712.02191 ancillary file (2017-12-06)
Supplement: Supplementary file 1 [file SI.pdf]

nature nanotechnology
SUPPLEMENTARY INFORMATION
DOI: 10.1038/NNANO.2017.111

In the format provided by the authors and unedited.

# Supplementary Information to "Monitoring the orientation of rare-earth doped nanorods for flow shear tomography"

J. Kim, S. Michelin, M. Hilbers, L. Martinelli, E. Chaudan, G. Amselem, J.-P. Boilot, A. M. Brouwer, C. Baroud, J. Peretti, and T. Gacoin

## I. EXPERIMENTAL PROCEDURES

### A. Measurement of photoluminescence spectra in transverse ($\sigma$, $\pi$) and homeotropic ($\alpha$) configurations

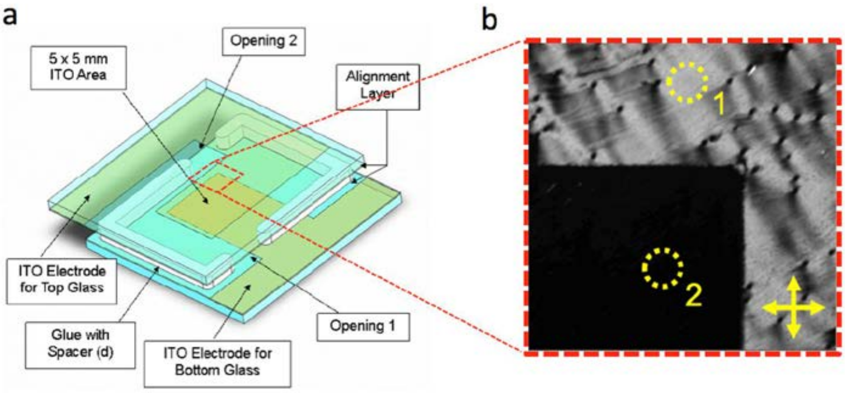


Supplementary Fig. S1. **Electro-optic measurements.** (a) Schematic of the homeotropic switching cell (Instec Inc, figure taken from the product brochure). (b) Optical transmission image (same as Figure 2d in the main script) between crossed polarizers (indicated by arrows) of the cell filled with a nematic $LaPO_4$:Eu nanorod suspension with an applied alternating electric field (1 V/m, 100 kHz). The image area is 1.8 mm $\times$ 1.8 mm.

### B. Sample preparation for single nanorod photoluminescence spectroscopy

For measuring the polarized luminescence spectra of a single nanorod of known size and orientation, the particles were deposited on a patterned substrate and a procedure was developed which allows to determine by AFM and SEM the rod dimensions as well as its position and orientation with respect to the pattern (Supplementary Figure S2).

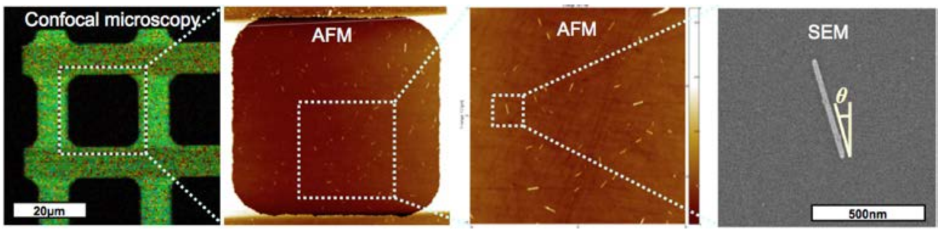


Supplementary Fig. S2. **Single nanorod sample preparation.** From left to right - Scanning confocal microscopy image of a quartz substrate with gold micro-grills on which the LaPO4:Eu nanorods were deposited; atomic force microscopy (AFM) image of a grid cell; AFM zoom image where individual nanorods are visible; SEM image of a single nanorod selected on the AFM image.



© 2017 Macmillan Publishers Limited, part of Springer Nature. All rights reserved.

## II. ANALYSIS OF THE LUMINESCENCE POLARIZATION

### A. Spectral deconvolution of sublevels

The deconvolution of the sublevels' contributions was based on the analysis of the polarized PL spectra collected from the aligned nanorods' film shown in Figure 2a of the main text. Focusing on the $^5D_0$-$^7F_1$ magnetic dipolar (MD) transition (Supplementary Figure S3.b), there exist three peaks at 587.5 nm, 590.7 nm, and 595.1 nm that correspond to the three degenerate sublevels and one satellite peak at 597.4 nm.

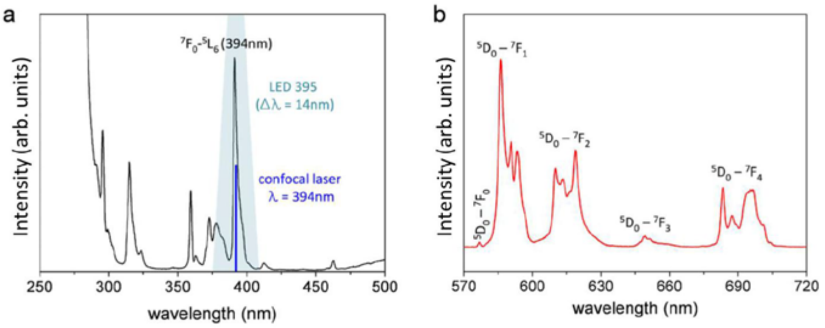


Supplementary Fig. S3. **Photoluminescence of LaPO4:Eu nanorods.**(a) Excitation spectrum of LaPO4:Eu nanorods obtained at the highest emission peak ($\lambda = 587.5$ nm). The blue region corresponds to the LED excitation source. The high absorption cross-section of the $^7F_0$-$^5L_6$ transition at the violet edge of the visible range (394 nm) allowed the use of standard optical apparatus for obtaining intense PL spectra. (b) Full emission spectrum of $LaPO_4$:Eu nanorods obtained under charge transfer band (CTB) excitation at 260 nm.

The peak deconvolution and fitting analysis were performed using the OPUS software. The best fitting peak lineshape was found to be 40%-Lorentzian and 60%-Gaussian. The spectral width of the LED excitation source (HWHM = 14 nm) broadly covering the narrow excitation peak of the $^7F_0$-$^5L_6$ transition (Supplementary Figure S3.a) seems to be responsible for the Gaussian broadening. Almost purely Lorentzian distribution was indeed found for the spectra taken with a narrow laser excitation source on the confocal microscope.

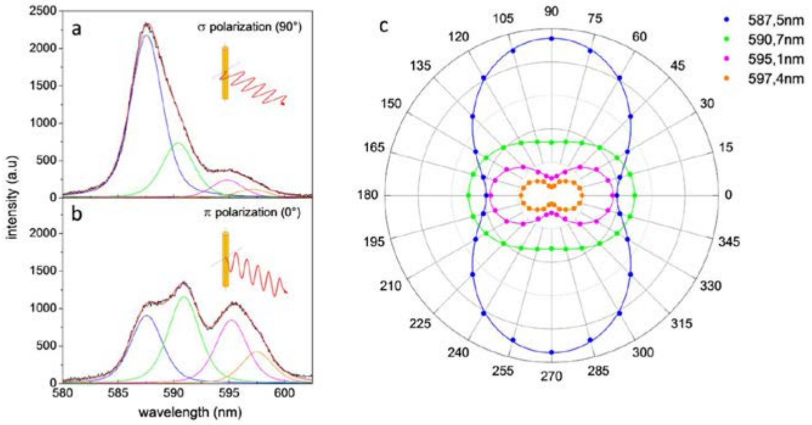


Supplementary Fig. S4. **Polarized photoluminescence of LaPO4:Eu nanorods.** $\sigma$-(a) and $\pi$-(b) polarized spectra on the $^5D_0$-$^7F_1$ MD transition with the fitted spectra (red line) as the sum of four deconvoluted peaks. (c) Polar diagram of the four peak intensities as a function of the analyzer angle varied by 15° steps corresponding to Figure 2a in the main text. The solid lines are dipolar fittings according to Eq. S1.


© 2017 Macmillan Publishers Limited, part of Springer Nature. All rights reserved.

The fitting result for the $\sigma$ and $\pi$ spectra plotted in (Supplementary Figure S4.a-b clearly shows the intensity of these four peaks vary in different way indicating the low symmetry of the $LaPO_4$:Eu crystals in the hexagonal rhabdophane phase. (Supplementary Figure S4.c is a polar diagram of the peak intensities taken at each 15° steps of the rotating analyzer. The discrete data points were fitted with the orthogonal dipolar components as:

$$I = A \cdot \sin^2\theta + B \cdot \cos^2\theta \qquad \text{(S1)}$$

where $I$ is the measured peak intensity and $\theta$ is the angle between the rod orientation and the polarizer.

The very good agreement between the fit and experimental data supports the deconvolution result. Supplementary Figure S5 shows each polar diagram together with the orthogonal dipolar components plotted as red lines. As described in the main text, $^5D_0$-$^7F_1$ is a magnetic dipolar transition level where the PL emission is polarized orthogonal to the magnetic dipolar axis. The $A$ and $B$ values and their standard errors obtained from the fitting analysis are noted in Table I. The angle $\psi$ between each dipole and the rod axis are also indicated. These angles reflect the dipolar geometry resulting from the crystal field splitting of sublevels. The very similar $\psi$ values for the peaks at 595.1 nm and 597.4 nm indicate that they originate from the same sublevel.

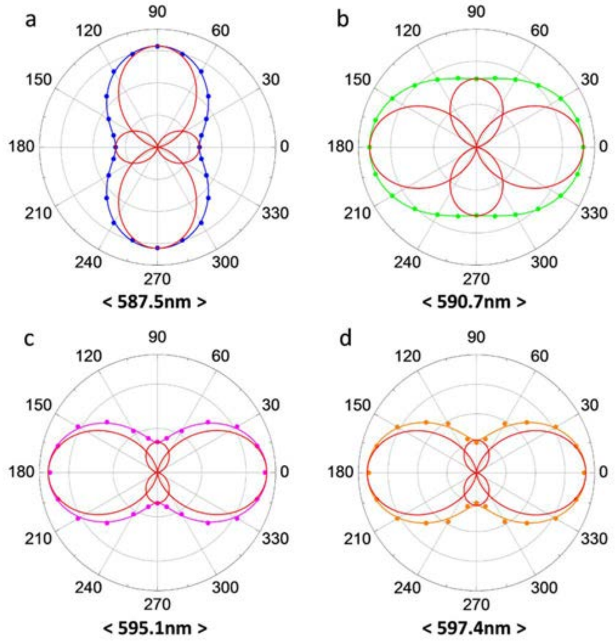


Supplementary Fig. S5. **Polar diagram of the intensity of the each peak of the $^5D_0$-$^7F_1$ MD transition.** The symbols correspond to the measurements and the full lines to the fits by two orthogonal dipolar components (red lines).

TABLE I. **dipolar components of the different contribution to the MD transition.** Intensities (in arbitrary units) and standard errors (S.E) of the orthogonal dipolar components ($A$, $B$) obtained from the fit of the polar emission diagram. The angle ($\psi$) between each dipole axis and the rod axis (crystallographic c-axis) is indicated.

| peak | 587.5 nm | 590.7 nm | 595.1 nm | 597.4 nm |
|---|---|---|---|---|
| $A$ | 9422 | 3191 | 1025 | 553 |
| S.E | 21.8 | 4.4 | 19.3 | 15.4 |
| $B$ | 3899 | 4979 | 3700 | 1852 |
| S.E | 20.7 | 4.2 | 18.3 | 14.6 |
| $\psi$ (deg.) | 67.5 | 32.7 | 15.5 | 16.6 |



© 2017 Macmillan Publishers Limited, part of Springer Nature. All rights reserved.

### B. Determination of the nanorod orientation

#### 1. Single nanorod

As demonstrated above, each sublevel transition dipole, with a particular angle $\psi$ with respect to the rod axis, can be decomposed into two orthogonal components parallel and perpendicular to the rod axis. Regarding the uniaxial crystalline symmetry of $LaPO_4$:Eu nanorod, the perpendicular component can be considered as two orthogonal components with an identical intensity for convenience (along the x and y axis on the plane perpendicular to the rod axis). Due to the different correlations among the $\sigma$, $\pi$, and $\alpha$ polarization components in the electric dipolar transition (ED) and the magnetic dipolar transition (MD) described in the main text, the total emission intensity of a nanorod can be expressed as:

$$\sum I_{ED} = 2I_\pi + 2I_\sigma + 2I_\alpha = 2I_\pi + 4I_\sigma \tag{S2}$$

$$\sum I_{MD} = 2I_\pi + 2I_\sigma + 2I_\alpha = 4I_\pi + 2I_\sigma \tag{S3}$$

Considering a nanorod with an orientation ($\theta$, $\varphi$) with respect to the laboratory frame as shown in Figure 2g of the main text, the intensities $I_{xz}$ and $I_{xy}$ of the polarization components along $z-$ and $y-$axis respectively, measured in the direction of observation along $x-$axis, can be expressed as a function of $I_\pi$ and $I_\sigma$.

For the ED emission, one obtains:

$$I_{xz} = I_\pi \cdot \cos^2\theta + I_\sigma \cdot \sin^2\theta \tag{S4}$$

$$I_{xy} = I_\pi \cdot \sin^2\theta \cdot \sin^2\varphi + I_\sigma \cdot \left(\cos^2\theta \cdot \sin^2\varphi + \cos^2\varphi\right) \tag{S5}$$

Then, fitting the full emission spectrum $I_{xy}(\lambda)$ by a linear combination of $I_\pi(\lambda)$ and $I_\sigma(\lambda)$ obtained from the measurement of a nematic nanorod suspension in an electro-optic cell, the $\theta$ value can be directly obtained using Eq. S4. Subsequently, the $\varphi$ value can be obtained from Eq. S5. It is also possible to selectively measure the emission intensities of different peaks (or bands) in the spectrum by using band path filters and a photo-detector. As each peak has a distinct polarization angle determined by the corresponding dipole orientation $\psi$ with respect to the rod c-axis, the fitting of the whole spectrum line shape can be replaced by the analysis of two selected peaks. For each peak (refered to as $n = 1$ or 2) Eq. S5 holds and relates $I_{nxy}$ to $I_{n\pi}$ and $I_{n\sigma}$. The value of $cos^2\theta$ can then be simply deduced from the ratio $k_{xz} = I_{1xz}/I_{2xz}$ according to the following equation :

$$cos^2\theta = \frac{k_{xz} \cdot I_{2\sigma} - I_{1\sigma}}{k_{xz} \cdot (I_{2\sigma} - I_{2\pi}) - (I_{1\sigma} - I_{1\pi})} \tag{S6}$$

Once the value of $cos^2\theta$ is obtained, the $cos^2\varphi$ value can be calculated in the same way using Eq. S5. There exist two symmetric orientations for each $\theta$ and $\varphi$ correponding to the obtained values of $cos^2\theta$ and $cos^2\varphi$. Measuring one more polarized spectra at an intermediate analysis angle between $x$- and $y$-axis (at 45° for example) enables to exclude two mirror images for $\varphi$. The elimination of the mirror image of $\theta$ requires one more measurement in another direction of observation. This is technically possible by tilting the sample or using a large aperture microscope objective with a diaphragm at different positions.

For the MD transitions, equations similar to Eqs. S4-S6 can be written (see Eq.1-2 in the main text),

$$I_{xz} = I_\sigma \cdot \sin^2\theta \cdot \sin^2\varphi + I_\pi \cdot \left(\cos^2\theta \cdot \sin^2\varphi + \cos^2\varphi\right) \tag{S7}$$

$$I_{xy} = I_\sigma \cdot \cos^2\theta + I_\pi \cdot \sin^2\theta \tag{S8}$$

In this case, $cos^2\theta$ can be deduced from the ratio $k_{xy} = I_{1xy}/I_{2xy}$ of two values of $I_{xy}$ measured at two different wavelength in the MD emission band:



© 2017 Macmillan Publishers Limited, part of Springer Nature. All rights reserved.

$$cos^2\theta = \frac{k_{xy} \cdot I_{2\pi} - I_{1\pi}}{k_{xy} \cdot (I_{2\pi} - I_{2\sigma}) - (I_{1\pi} - I_{1\sigma})} \tag{S9}$$

Therefore, both ED and MD emission can be used to detect the orientation of a single nanorod.

### 2. *Partially oriented nanorods suspension* $(0 < f < 1)$ *along a known director* $\vec{n}$

The orientation state of a colloidal suspension containing many nanorods is defined by two quantities: the order parameter $f$ and its director $\vec{n}$. The order parameter quantifies the local dispersion in the particle's orientation : $f = 1$ when all particles have locally the same orientation, while $f = 0$ for a fully disordered system. The observed polarized emission spectra from a local volume is an averaged sum of the emission from all the nanorods residing in the volume that have a certain orientation distribution in $\theta$ and $\varphi$ with respect to $\vec{n}$. When the nanorods are submitted to an external field such as electric field or flow shear, or oriented by the spontaneous LC organization, $\vec{n}$ can often be found directly from the direction of the external field. In this case, two polarization components parallel and perpendicular to $\vec{n}$ can be noted as $I_{\parallel}$ and $I_{\perp}$ (Figure 2h in the main text) which have the same form as $I_{xz}$ and $I_{xy}$ for the case of a single nanorod.

For the ED emission, one has:

$$I_{\parallel} = \langle I_\pi \cdot \cos^2\theta + I_\sigma \cdot \sin^2\theta \rangle \tag{S10}$$

$$I_{\perp} = \langle I_\pi \cdot \sin^2\theta \cdot \sin^2\varphi + I_\sigma \cdot \left(\cos^2\theta \cdot \sin^2\varphi + \cos^2\varphi\right) \rangle \tag{S11}$$

where the sign $\langle\ \rangle$ stands for the average over many nanorods. Since $\vec{n}$ is a cylindrical symmetry axis, $\langle sin^2\varphi \rangle = \langle cos^2\varphi \rangle = 1/2$ and thus Eqs. S10 and S11 can be written as:

$$I_{\parallel} = I_\pi \cdot \langle cos^2\theta \rangle + I_\sigma \cdot \left(1 - \langle cos^2\theta \rangle\right) \tag{S12}$$

$$I_{\perp} = \frac{I_\pi}{2} \cdot \left(1 - \langle cos^2\theta \rangle\right) + \frac{I_\sigma}{2} \cdot \left(1 + \langle cos^2\theta \rangle\right) \tag{S13}$$

The $\langle cos^2\theta \rangle$ value can then be obtained in the same way as the value of $cos^2\theta$ for a single nanorod using $k_{\parallel} = I_{1\parallel}/I_{2\parallel}$, the ratio of two values of $I_{\parallel}$ measured at two different emission wavelength:

$$\langle cos^2\theta \rangle = \frac{k_{\parallel} \cdot I_{2\sigma} - I_{1\sigma}}{k_{\parallel} \cdot (I_{2\sigma} - I_{2\pi}) - (I_{1\sigma} - I_{1\pi})} \tag{S14}$$

For the MD emission, similar equations, shown as Eqs. 3-4 in the main text, can be written:

$$I_{\parallel} = \frac{I_\sigma}{2} \cdot \left(1 - \langle cos^2\theta \rangle\right) + \frac{I_\pi}{2} \cdot \left(1 + \langle cos^2\theta \rangle\right) \tag{S15}$$

$$I_{\perp} = I_\sigma \cdot \langle cos^2\theta \rangle + I_\pi \cdot \left(1 - \langle cos^2\theta \rangle\right) \tag{S16}$$

And again $\langle cos^2\theta \rangle$ can be deduced from the ratio $k_{\parallel}$ of two values of $I_{\parallel}$:

$$\langle cos^2\theta \rangle = \frac{k_{\parallel} \cdot (I_{2\sigma} + I_{2\pi}) - (I_{1\sigma} + I_{1\pi})}{k_{\parallel} \cdot (I_{2\sigma} - I_{2\pi}) - (I_{1\sigma} - I_{1\pi})} \tag{S17}$$

Then, from the obtained value of $\langle cos^2\theta \rangle$, one can deduce the value of $f = \left(3\langle cos^2\theta \rangle - 1\right)/2$.



© 2017 Macmillan Publishers Limited, part of Springer Nature. All rights reserved.

### 3. General solution for unknown order parameter $f$ and unknown director $\vec{n}$

When $\vec{n}$ is unknown, the angular orientation of $\vec{n}$ with respect to the laboratory frame ($\theta'$, $\varphi'$) has first to be determined. The measured polarized PL intensities, $I_{xz}$ and $I_{xy}$, can be expressed as a function of $I_{\parallel}$ and $I_{\perp}$ defined above in the form of equations similar to Eqs. S4-S5. For both ED and MD emission, one gets:

$$I_{xz} = I_{\parallel} \cdot \cos^2\theta' + I_{\perp} \cdot \sin^2\theta' \tag{S18}$$

$$I_{xy} = I_{\parallel} \cdot \sin^2\theta' \cdot \sin^2\varphi' + I_{\perp} \cdot \left(\cos^2\theta' \cdot \sin^2\varphi' + \cos^2\varphi'\right) \tag{S19}$$

For ED emission, by substituting Eqs. S12-S13 in Eq. S18, one obtains:

$$I_{xz} = \frac{I_{\pi}}{2} \cdot \left(1 - \langle\cos^2\theta\rangle - \cos^2\theta' + 3\langle\cos^2\theta\rangle \cdot \cos^2\theta'\right) + \frac{I_{\sigma}}{2} \cdot \left(1 + \langle\cos^2\theta\rangle + \cos^2\theta' - 3\langle\cos^2\theta\rangle \cdot \cos^2\theta'\right) \tag{S20}$$

Similarly to Eq. S6, the intensity ratio of two distinct peaks in one spectrum ($k_{xz} = I_{1xz}/I_{2xz}$) provides the following equation for $\langle\cos^2\theta\rangle$ and $\cos^2\theta'$:

$$\langle\cos^2\theta\rangle + \cos^2\theta' - 3\langle\cos^2\theta\rangle \cdot \cos^2\theta' = -\frac{k\,(I_{2\sigma} + I_{2\pi}) - (I_{1\sigma} + I_{1\pi})}{k\,(I_{2\sigma} - I_{2\pi}) - (I_{1\sigma} - I_{1\pi})} \tag{S21}$$

For MD emission, by substituting in Eq. S18 the expressions $I_{\parallel}$ and $I_{\perp}$ given by Eqs. S15-S16, one obtains:

$$I_{xz} = \frac{I_{\sigma}}{2} \cdot \left(2\langle\cos^2\theta\rangle + \cos^2\theta' - 3\langle\cos^2\theta\rangle \cdot \cos^2\theta'\right) + \frac{I_{\pi}}{2} \cdot \left(2 - 2\langle\cos^2\theta\rangle - \cos^2\theta' + 3\langle\cos^2\theta\rangle \cdot \cos^2\theta'\right) \tag{S22}$$

$$2\langle\cos^2\theta\rangle + \cos^2\theta' - 3\langle\cos^2\theta\rangle \cdot \cos^2\theta' = -2 \cdot \frac{k_{xz} \cdot I_{2\pi} - I_{1\pi}}{k_{xz} \cdot (I_{2\sigma} - I_{2\pi}) - (I_{1\sigma} - I_{1\pi})} \tag{S23}$$

Therefore, the two unknown values of $\langle\cos^2\theta\rangle$ and $\cos^2\theta'$ can be determined from Eqs. S21 and S23 from ED and MD. The value of $\cos^2\varphi'$ can then be calculated using Eq. S19. Finally, the mirror values of $\varphi'$ can be eliminated in the same way as indicated for the case of a single nanorod.

### 4. Calculation of $f$ and $\vec{n}$ on the microfluidic channel cross-sections

The determination of $f$ and $\vec{n}$ from experiments performed in a microfluidic channel with a constriction as described in the main text was achieved using the above equations that were simplified taking into account the boundary conditions. Polarized PL measurements on a single transition level (preferably a MD transition that exhibits more dramatic line shape change than an ED transition) provides sufficient information. In the case of the vertical section (Figure 4a, 4c-left, and 4d in the main text), as $\vec{n}$ is constantly normal to the scanning plane, Eqs. S15-S16 were used to obtain $\langle\cos^2\theta\rangle$ and $f$. In the case of the horizontal section across the constriction (Figure 4a, 4c-right, and 4e in the main text) located at the middle height of the channel, the value of $\varphi'$ is fixed at 90° and thus Eq. S19 simplifies as:

$$I_{xy} = I_{\parallel} \cdot \sin^2\theta' + I_{\perp} \cdot \cos^2\theta' \tag{S24}$$



© 2017 Macmillan Publishers Limited, part of Springer Nature. All rights reserved.

To eliminate the mirror images of $\varphi'$, an additional equation for the measurement at the analyzer angle of 45° can be expressed as:

$$\begin{aligned} I_{x45^\circ} = I_{\parallel} \cdot \cos^2\left(\frac{\pi}{4} - \theta'\right) + I_{\perp} \cdot \sin^2\left(\frac{\pi}{4} - \theta'\right) \\ = \frac{I_{\parallel}}{2} \cdot (1 + sin2\theta') + \frac{I_{\perp}}{2} \cdot (1 - sin2\theta') \\ = \frac{I_{\parallel} + I_{\perp}}{2} + sin2\theta' \cdot \frac{I_{\parallel} - I_{\perp}}{2} \end{aligned} \quad \text{(S25)}$$

From Eq. S18 and S25 one can obtain:

$$tan2\theta' = \frac{2I_{x45^\circ} - I_{xz} - I_{xy}}{I_{xz} - I_{xy}} \quad \text{(S26)}$$

Considering $\theta'$ ranges between 90° and −90°, the solution for $\theta'$ can be expressed as:

$$\theta' = \frac{1}{2}\left[arctan\,(\Sigma) - \frac{\pi}{2} \cdot \frac{\Sigma}{|\Sigma|}\left(\frac{\Gamma}{|\Gamma|} + 1\right)\right] \quad \text{(S27)}$$

where,

$$\Sigma = \frac{2I_{x45^\circ} - I_{xz} - I_{xy}}{I_{xz} - I_{xy}} \quad \text{and} \quad \Gamma = I_{xz} - I_{xy}$$

The values of $I_{\parallel}$ and $I_{\perp}$ were obtained with the value of $\theta'$ using Eq. S18 and S24. The values of $\langle\cos^2\theta\rangle$ and $f$ were then obtained using Eq. S15-S16.

### C. Determination of the apparent shear rate $\dot{\gamma}_{\text{app}}$

The apparent shear rate at each focal point in the microfluidic channel can be deduced from the value of $f$ using the stress optical law shown in Supplementary Figure S6a. This curve is obtained by fitting the experimental (polarized luminescence and birefringence) data obtained on a linear microfluidic channel with the model described in the next section (see Figure 3f in the main text).

The uncertainty $\Delta\dot{\gamma}_{\text{app}}$ on the determination of $\dot{\gamma}_{\text{app}}$ is related to the uncertainty $\Delta f$ on the experimental determination of $f$ by the slope of the stress optical law:

$$\Delta\left(\dot{\gamma}_{\text{app}}/\Omega\right) = \frac{\partial\left(\dot{\gamma}_{\text{app}}/\Omega\right)}{\partial f}\Delta f. \quad \text{(S28)}$$

The sensitivity of the measurement to the value of the apparent shear rate is then characterized by the ratio:

$$\frac{\dot{\gamma}_{\text{app}}}{\Delta\dot{\gamma}_{\text{app}}} = \frac{F}{\Delta f} \quad \text{(S29)}$$

where

$$F = \left(\dot{\gamma}_{\text{app}}/\Omega\right) \cdot \frac{\partial f}{\partial\left(\dot{\gamma}_{\text{app}}/\Omega\right)} \quad \text{(S30)}$$

defines the figure of merit for the determination of the apparent shear rate (Supplementary Figure S6b).



© 2017 Macmillan Publishers Limited, part of Springer Nature. All rights reserved.

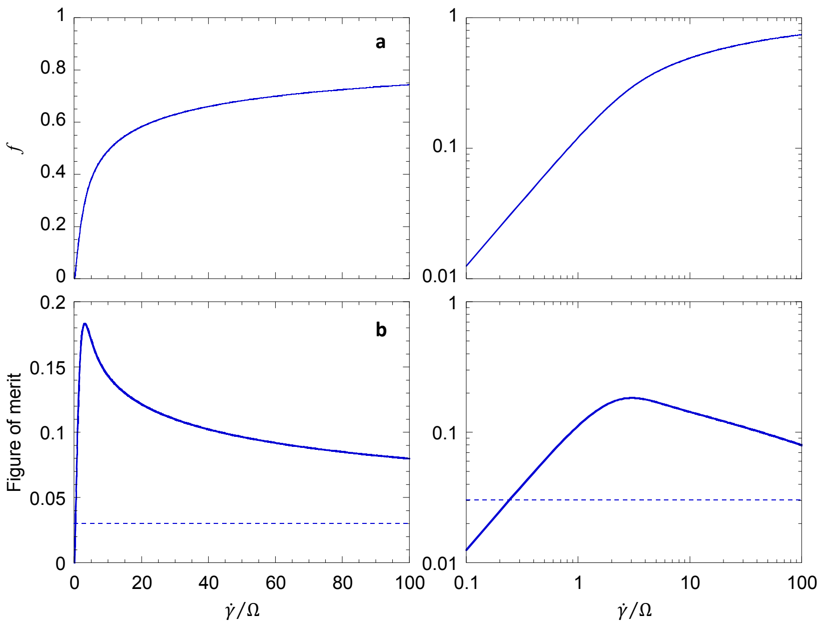


Supplementary Fig. S6. **Relation between the apparent shear rate and the order parameter.**(a) Order parameter $f$ as a function of the shear-rate-to-diffusion ratio for a plane parallel shear flow. (b) Figure of merit $F$ for the experimental determination of the apparent shear rate. log-log plots of the same quantities are also shown (right).

From the expressions of $\langle\cos^2\theta\rangle$ given in the previous sections, it can easily be shown that:

$$\Delta f \approx \frac{\Delta I}{I} \tag{S31}$$

where $I$ is the number of photons detected at a single focal point of the 3D photoluminescence mapping of the channel in a narrow band around the chosen transition wavelength (for instance, $I = I_{1xz}$). In the experiment reported here, the typical value of $I$ is of the order of a few 1000 for the highest resolution (the probed confocal volume is $\sim 1\ \mu m^3$) and measurements are shot-noise limited. Therefore, $\Delta f \approx 1/\sqrt{I} \approx 1/30$ (dashed line in Supplementary Figure S6b) and the ratio $\dot{\gamma}_{\rm app}/\Delta\dot{\gamma}_{\rm app}$ is larger than unity over a range. When downgrading the resolution by about a factor of 2, the probed volume and the number of detected photons increase by about an order of magnitude and the uncertainty on the determination of the shear rate becomes less than 10% for $\dot{\gamma}_{\rm app}/\Omega$ ranging from 0.1 to several 100 (while, in the present case, the fitting of the stress-optical law gives $\Omega = 0.5\ s^{-1}$).

## III. MODELING THE SHEAR FLOW AND THE PARTICLE ORIENTATION

### A. Particle reorientation in viscous flows

A simplified two-dimensional model is proposed here for the particle reorientation dynamics in the geometry of Figure 4 of the main text, based on two main assumptions: (i) the flow is purely two-dimensional and (ii) each particle (i.e. slender rods of length $a$ and diameter $b$ with $\rho = a/b \gg 1$) lies in the $(x, y)$ shear plane, its orientation being defined by its polar angle $\varphi$ (see Supplementary Figure S7).

For a small rod-like particle (i.e. $b \ll a \ll H$), the evolution of $\varphi$ is described as (Jeffery's orbits, [2])

$$\dot{\varphi} = \frac{\omega + \dot{\gamma}\cos(2\varphi - 2\Phi)}{2}, \tag{S32}$$



© 2017 Macmillan Publishers Limited, part of Springer Nature. All rights reserved.

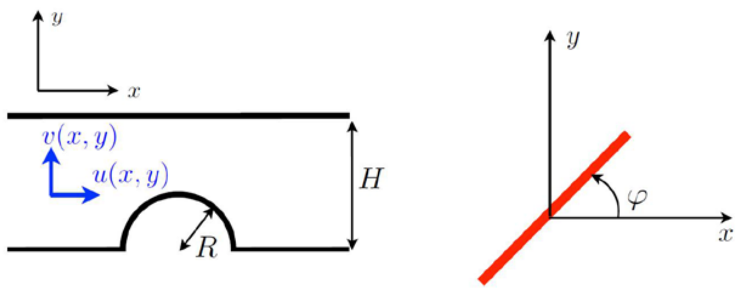


Supplementary Fig. S7. **Definition of the particle's orientation.**

where $\omega(x, y)$, $\Phi(x, y)$ and $\dot{\gamma}(x, y)$ are the local vorticity, principal shear direction and modulus, respectively:

$$\omega = \frac{\partial v}{\partial x} - \frac{\partial u}{\partial y}, \quad \dot{\gamma} = \sqrt{\left(\frac{\partial u}{\partial x} - \frac{\partial v}{\partial y}\right)^2 + \left(\frac{\partial u}{\partial y} + \frac{\partial v}{\partial x}\right)^2}. \tag{S33}$$

### B. Reorientation dynamics in a dilute suspension

For dilute suspensions of such particles in steady flows, the probability density function $\psi(x, y, \varphi)$ to find a particle at location $(x, y)$ with orientation $\varphi$ satisfies [4]

$$\mathbf{u} \cdot \nabla\psi + \frac{\partial}{\partial\varphi}(\psi\dot{\varphi}) = \Omega\, \frac{\partial^2\psi}{\partial\varphi^2}, \tag{S34}$$

where the different terms describe the advection of the particles by the flow, their reorientation by the flow gradient, and their rotational diffusion. $\Omega$ is the particles' rotational diffusivity (see Eq. (5) of main text); translational diffusion is negligible here since $a \ll H$.

The order parameter, $f$, is obtained from $\psi$ as:

$$f(x, y) = \sqrt{< \sin(2\varphi) >_\varphi^2 + < \cos(2\varphi) >_\varphi^2}. \tag{S35}$$

In a straight channel, $\mathbf{u} \cdot \nabla\psi = 0$, and the reorientation of particles in shear balances rotational diffusion:

$$\frac{\partial}{\partial\varphi}\left[\psi\left(\frac{\omega + \dot{\gamma}\cos(2\varphi - 2\bar{\varphi})}{2}\right)\right] = \Omega\, \frac{\partial^2\psi}{\partial\varphi^2}. \tag{S36}$$

The order parameter $f$ then depends solely on the *local* flow vorticity $\omega$ and shear $\dot{\gamma}$. Further, for such parallel flows, $\omega = -\dot{\gamma}$, and the order parameter is a function of $\dot{\gamma}$ only: $f = g(\dot{\gamma}/\Omega)$. The resulting stress-optical law ([1], Supplementary Figure S6) can be inverted to obtain an estimation of the apparent shear rate $\dot{\gamma}_{\text{app}}$:

$$\dot{\gamma}_{\text{app}} = \Omega\; g^{-1}(f). \tag{S37}$$

In more complex geometries, particles' advection leads to a change in the flow experienced by each particle on a typical time scale $H/U$, to be compared to the rotational diffusion time scale $\Omega^{-1}$. Their ratio is the Péclet number $\text{Pe} = U/\Omega H$ and is a measure of the relative effect of advection and diffusion.

For fast diffusion ($\text{Pe} \ll 1$), the particles' orientation adjusts instantaneously; Eqs. (S36) and (S37) remain valid.



© 2017 Macmillan Publishers Limited, part of Springer Nature. All rights reserved.

For slow diffusion, (Pe $= O(1)$), the full dynamics must be considered and Eq. (S34) must be solved. $f$ now depends on the history of the flow experienced by the particles, and not only on the local flow conditions. Finding $f$ and $\dot{\gamma}_{\text{app}}$ now proceeds in two steps:

- first, find the flow velocity $\mathbf{u}$ everywhere in a given channel, its gradient, as well as the flow streamlines;
- second, solve Eq. (S34) as an evolution equation for $\psi$ along each streamline, to obtain $\psi$ and $f$ everywhere.

### C. Flow computations

The flow field is computed using a Boundary Integral Method [3], in a fluid domain $V_f$ corresponding to the section $-L \leq x \leq L$ of the channel of Supplementary Figure S7 ($x = 0$ corresponds to the center of the obstacle, and $L \gg H$). The flow velocity $\mathbf{u}$ satisfies the integral equation:

$$\alpha \mathbf{u}(\mathbf{x}) = \int_{\partial V_f} [\mathbf{S}(\mathbf{r}) \cdot \mathbf{f}(\mathbf{x}') - \mathbf{u}(\mathbf{x}') \cdot \mathbf{T}(\mathbf{r}) \cdot \mathbf{n}(\mathbf{x}')] \, dl(\mathbf{x}') \quad \text{(S38)}$$

with $\mathbf{r} = \mathbf{x} - \mathbf{x}'$, and $\alpha = 1$ (resp. $\alpha = 1/2$) for a point inside (resp. on the boundary of) the domain. $\mathbf{S}$ and $\mathbf{T}$ are the single- and double-layer potentials, respectively:

$$\mathbf{S}(\mathbf{r}) = \frac{1}{2\pi}\left(\mathbf{I}\log(r) - \frac{\mathbf{rr}}{r^2}\right), \quad \mathbf{T}(\mathbf{r}) = \frac{4\,\mathbf{rrr}}{r^4}. \quad \text{(S39)}$$

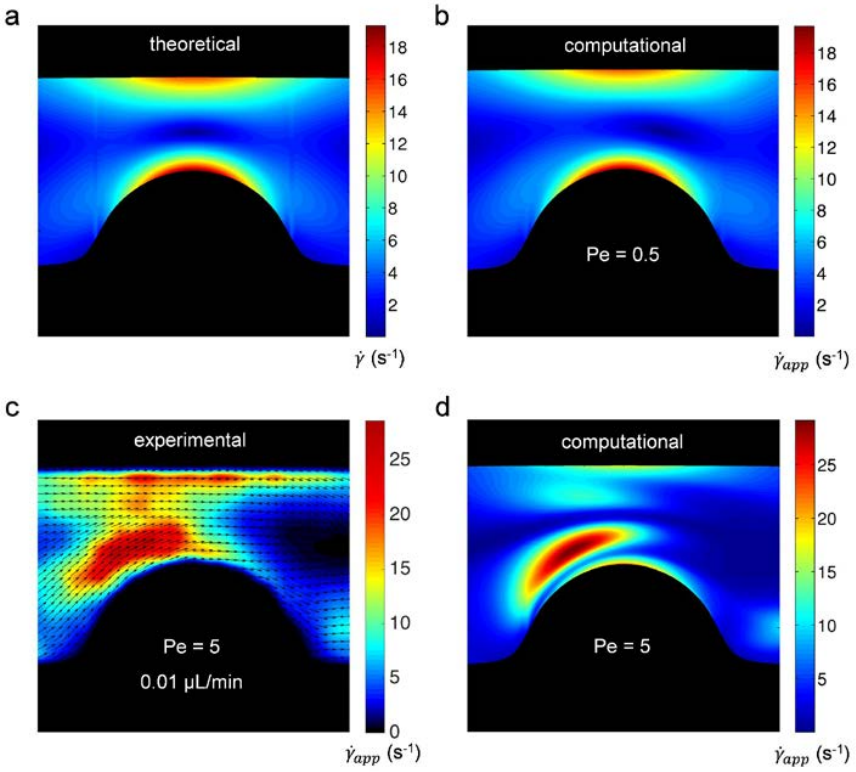


Supplementary Fig. S8. **Apparent and Actual shear rates.** Apparent shear (in $s^{-1}$) from the distribution of order parameter (a) measured for Pe = 5, (b) calculated for Pe = 5 and (d) for Pe = 0.5. (c) Actual shear rate $\dot{\gamma}$ ($s^{-1}$) around the obstacle calculated for the experimental conditions $H = 50\mu$m and $U = 140\mu$m.s$^{-1}$.



© 2017 Macmillan Publishers Limited, part of Springer Nature. All rights reserved.

Applying Eq. (S38) on $\partial V_f$ provides an integral equation for the boundary flow velocity and traction forces $\mathbf{f}$, which is inverted numerically by imposing no-slip ($\mathbf{u} = 0$) on the solid walls, a horizontal inlet/outlet flow velocity and a fixed pressure drop $\Delta p$ between $x = \pm L$.

The flow velocity and its gradient are computed anywhere in $V_f$ using Eq. (S38) and $\dot{\gamma}$ is found from Eq. (S33). The shear rate intensity is symmetric about the obstacle (Supplementary Figure S8a). The position of a given streamline $\mathbf{x}_s(s)$ is found by solving $\mathbf{u}(\mathbf{x}_s) \times \partial \mathbf{x}_s / \partial s = 0$.

### D. Determination of the particle orientation in the channel

Equation (S34) is then solved along each streamline numerically using an implicit second order finite difference scheme. The initial condition at $x = -L$ is obtained from the classical straight channel results. From $\psi$, the distribution of order parameter in the entire channel and the apparent shear rate are computed using Eqs. (S35) and (S37) for different Pe (Supplementary Figure S8b and d).

For low Pe (small particles), $\dot{\gamma}_{\text{app}}$ (Supplementary Figure S8b) closely matches the actual shear rate (Supplementary Figure S8a) confirming that the quasi-steady analysis is valid. For slower diffusion (larger particles), $\dot{\gamma}_{\text{app}}$ (Supplementary Figure S8d) and $\dot{\gamma}$ (Supplementary Figure S8a) do not match anymore (in particular, $\dot{\gamma}_{\text{app}}$ is not symmetric around the obstacle as opposed to $\dot{\gamma}$). Nevertheless the simulated $\dot{\gamma}_{\text{app}}$ (Supplementary Figure S8d) matches very well the experimental observations (Supplementary Figure S8c).


[1] J. T. Edsall H. A. Scheraga and J. O. Gadd. Double refraction of flow: numerical evaluation of extinction angle and bi-refringence as a function of velocity gradient. *J. Chem. Phys.*, 19:1101, 1951.
[2] G. B. Jeffery. The motion of ellipsoidal particles immersed in a viscous fluid. *Proc. Roy. Soc. A*, 102:161–179, 1922.
[3] C. Pozrikidis. *Boundary integral and singularity methods for linearized viscous flows.* Cambridge Univ. Press, Cambridge, 1992.
[4] D. Saintillan and M. J. Shelley. Instabilities, pattern formation and mixing in active particle suspensions. *Phys. Fluids*, 20:123304, 2008.




© 2017 Macmillan Publishers Limited, part of Springer Nature. All rights reserved.
